# Supplementary material for: Giant Frictional Drag in Double Bilayer Graphene Heterostructures
Source: arXiv:1603.00757 ancillary file (2016-03-02)
Supplement: Supplementary file 1 [file SM.pdf]

# Supplementary Material for

## Frictional Drag in Double Bilayer Graphene Heterostructures

Kayoung Lee, Jiamin Xue, David C. Dillen,
Kenji Watanabe, Takashi Taniguchi, and Emanuel Tutuc

correspondence to: etutuc@mer.utexas.edu

Layer and drag measurements in double bilayer graphene heterostructures

Four-point resistance measurements were performed on the bottom and top bilayer graphene by flowing source currents of 1 nA on each bilayer using lock-in amplifiers, as described in Ref. [S1]. Different lock-in frequencies, ranging between 7 – 17 Hz were chosen for the bottom and top bilayers to exclude the cross-talk between the two bilayers. A radio-frequency transformer (Jensen Transformers, model JT-SUB-BB) is used to flow AC currents on the top bilayer, while applying a DC bias $V_{TL}$ with respect to ground. Samples were measured in a variable-temperature liquid $^4$He flow cryostat, which provides temperature ($T$) down to 1.5 K.

Coulomb drag measurements were performed either on the bottom or top bilayer graphene, separately. While flowing an AC drive current $I_{Drive}$ of 1 – 10 nA on the drive layer, we measure the four-point drag voltage $V_{Drag}$ in the opposite, drag layer [S2]. The drag resistance $R_{Drag}$ is then defined as $V_{Drag}/I_{Drive}$. Conventional lock-ins are used to flow AC drive currents, and to measure the AC drag voltages, where the lock-in frequencies for the bottom and top bilayers are synchronized. The drag resistances were also probed by flowing DC drive currents; we flow DC drive current by applying a DC voltage on the drive layer, and measure a voltage drop in the opposite, drag layer. $R_{Drag}$ is then defined as $dV_{Drag}/dI_{Drive}$ in the limit of $I_{Drive} = 0$. $R_{Drag}$ from the $dV_{Drag}/dI_{Drive}$ agrees with $R_{Drag}$ measured using lock-ins.

Carrier density calculation in double bilayer graphene heterostructures

The detailed gate-depending characteristics of each bilayer graphene, without the crosstalk between the two bilayers, in double bilayer graphene heterostructures are discussed in Ref. [S1]. The bottom ($n_B$) and top ($n_T$) bilayer densities and gate biases have the following relations:

$$eV_{BG} = e^2(n_B + n_T)/C_{BG} + \mu_B \quad \text{(S1)}$$
$$eV_{TL} = -e^2 n_T/C_{int} - \mu_T + \mu_B \quad \text{(S2)}$$

Here, $C_{BG}$ and $C_{int}$ are the back-gate and interlayer dielectric capacitances, whereas $\mu_B$ and $\mu_T$ are the chemical potentials (Fermi energies, $\mu$) of the bottom and top bilayers, respectively; $e$ is the electron charge. $\mu$ and $n$ are positive (negative) for electrons (holes), and $V_{BG}$ and $V_{TL}$ in Eqs. S1 and S2 are referenced with respect to the bias values at $n_B = n_T = 0$ (double neutrality point, DNP).

Our previous studies in double bilayer graphene heterostructures probe experimentally the chemical potential in bilayer graphene [S1]. Figure S1 shows the $\mu$ vs. $n$ measured in multiple double bilayer graphene samples. Fitting to the measured $\mu$ in Sample A using a polynomial function provides the following formula describing $\mu$ as a function of carrier density $n$.

$$\mu(n) = 0.357n + 0.208n^2 - 0.884n^3 - 2.23n^4 + 2.98n^5 \quad \text{(S3)}$$

valid in the range of $-0.3 < n < 0.3$, where $n$ is expressed in unit of $10^{13}$ cm$^{-2}$, and $\mu$ is in unit of eV. While only a fit to the experimental data, this $\mu$ vs. $n$ dependence for bilayer graphene in Eq. (S3) is useful in solving Eqs. (S1) and (S2) self-consistently. Figure S2(a,b) presents the calculated $n_B$ and $n_T$ as a function of $V_{BG}$ and $V_{TL}$ for Sample A.

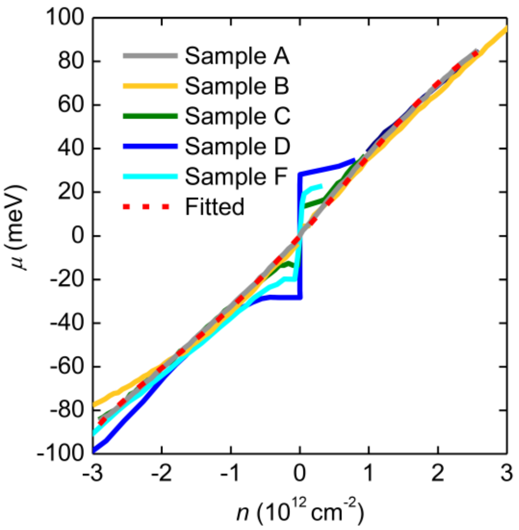


**Fig. S1**.

$\mu$ vs. $n$ in bilayer graphene, measured using our double bilayer graphene heterostructures as presented in Ref. [S1].

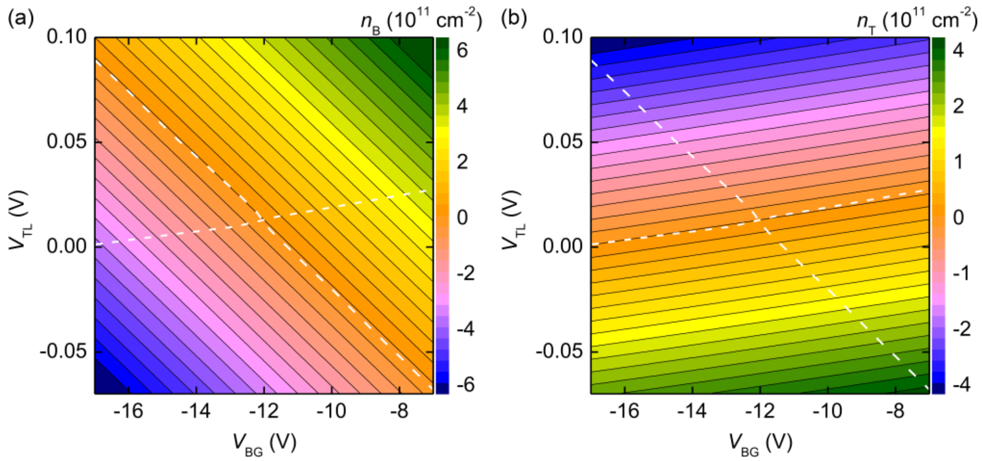


**Fig. S2**

(a) $n_B$ and (b) $n_T$ calculated as a function of $V_{BG}$ and $V_{TL}$ for Sample A. The white dashed lines represent the measured charge neutrality of the bottom and top bilayer graphene.

Electric field calculation in double bilayer graphene heterostructures

The transverse electric fields ($E$) across the bottom ($E_B$) and top ($E_T$) bilayer graphene can be described as [S3]

$$E_B = en_B/2\varepsilon_0 + en_T/\varepsilon_0 + E_{B0} \quad (S4)$$
$$E_T = en_T/2\varepsilon_0 + E_{T0} \quad (S5)$$

, where $\varepsilon_0$ is the vacuum permittivity, and $E_{B0}$ ($E_{T0}$) is the $E$ value in the bottom (top) bilayer graphene at DNP by an unintentional doping. In the bottom bilayer graphene, $n_B = 0$ and $E_B = 0$ point is identified by the Dirac point with the lowest resistance, as marked in Fig. 1(b). Eq. (S4) at $n_B = 0$ and $E_B = 0$ can be written as

$$E_{B0} = -en_T/\varepsilon_0 = C_{BG}\Delta V_{BG}/\varepsilon_0 \quad (S6)$$

, where $\Delta V_{BG}$ is the difference between the $V_{BG}$ values at DNP and at the $n_B = 0$ and $E_B = 0$ point. However, $E_{T0}$ cannot be calculated in the similar manner.

We estimate $E_{T0}$ using two different methods. For the low mobility top bilayer graphene, not encapsulated by hexagonal boron nitride (hBN), $E_{T0}$ is approximated as introduced in Ref. [S3]. Here, we presume the dopants, which move DNP from $V_{BG} = 0$ and $V_{TL} = 0$, are mostly located on top of the top bilayer graphene. Gauss law then provides

$$E_{T0} = C_{BG}V_{BG\_DNP}/\varepsilon_0 \quad (S7)$$

where $V_{BG\_DNP}$ is the $V_{BG}$ value at DNP.

For the higher quality double bilayer graphene heterostructures, encapsulated by hBN with high top and bottom bilayer mobilities, we estimate the $E$-field by measuring the transport gap as discussed in Ref. [S4]. Bilayer graphene exhibits a transverse $E$-field induced band gap [S5]. At a finite $E$-field in bilayer graphene, its conductivity shows finite threshold voltages along the electron and hole branches, analogous to the threshold voltages seen in a gapped semiconductor. The transport gap can be extracted from the threshold voltages, and Ref. [S4] shows the gap extraction in dual-gated bilayer graphene with oxide dielectrics. This method is employed here to estimate the gap, and the corresponding $E$ value at DNP in the bottom and top bilayer graphene in our double bilayer graphene heterostructures. The obtained $E_{B0}$ and $E_{T0}$ are given in Table S1. Using Eq. (S4) and Eq. (S5), along with the $E_{B0}$ and $E_{T0}$ values, $E_B$ and $E_T$ are calculated as a function of $n_B$ and $n_T$, which are related to the applied $V_{BG}$ and $V_{TL}$ as presented in Fig. S2. Figure S3 shows the calculated $E_B$ and $E_T$ as a function of $V_{BG}$ and $V_{TL}$ in Sample A.

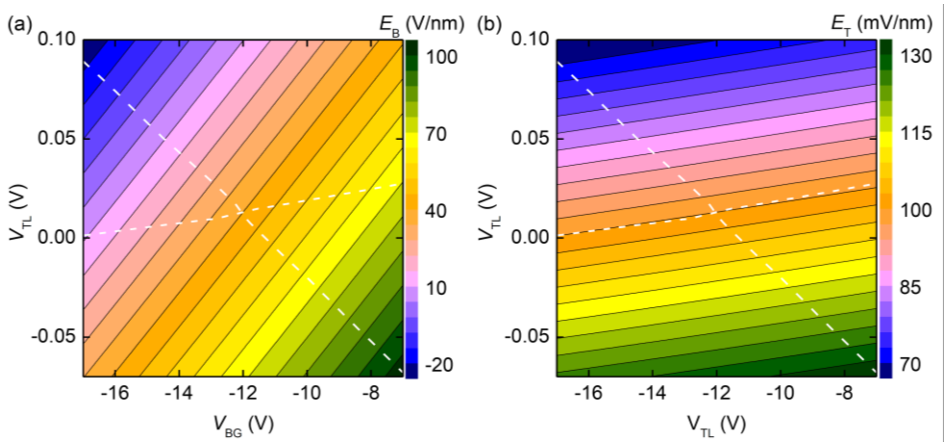


**Fig. S3**

(a) $E_B$ and (b) $E_T$ in Sample A calculated as a function of $V_{BG}$ and $V_{TL}$. The white dashed lines show the measured charge neutrality of the bottom and top bilayer graphene.

Magnetotransport properties of the bottom and top bilayer graphene

In a high perpendicular magnetic field ($B$ = 12 T), the longitudinal resistance in each bottom and top bilayer [Fig. S4(a,b)] shows minima at all integer filling factors $|\nu|$ up to 8 in the bottom bilayer, and up to 4 in the top bilayer, respectively. This indicates clearly developed integer quantum Hall states with full spin and valley degeneracy lifting in bilayer graphene. Further detailed studies on quantum Hall ferromagnetism in bilayer graphene may be found in Ref. [S1]. We note that the $V_{TL}$ spacing between adjacent quantum Hall states is not exactly identical because of the finite quantum capacitances of the two bilayers. Fig. S4(c) shows the contour map of the top bilayer longitudinal resistance ($R_{Top}$) as a function of $V_{BG}$ and $V_{TL}$, at $B$ = 12 T. The charge neutrality points (the red locus) show clear jumps in the change of $V_{TL}$ at finite $V_{BG}$ values, because $V_{TL}$ is used to move the bottom bilayer chemical potential to the next quantized LL (more details in Ref. [S1]). The large $V_{TL}$ jumps represents the gaps at $\nu = \pm4$, and smaller jumps are visible at $\nu = \pm1, \pm2, \pm3$ gaps, as marked. The clearly developed integer quantum Hall states confirm the high quality of our double bilayer graphene samples.

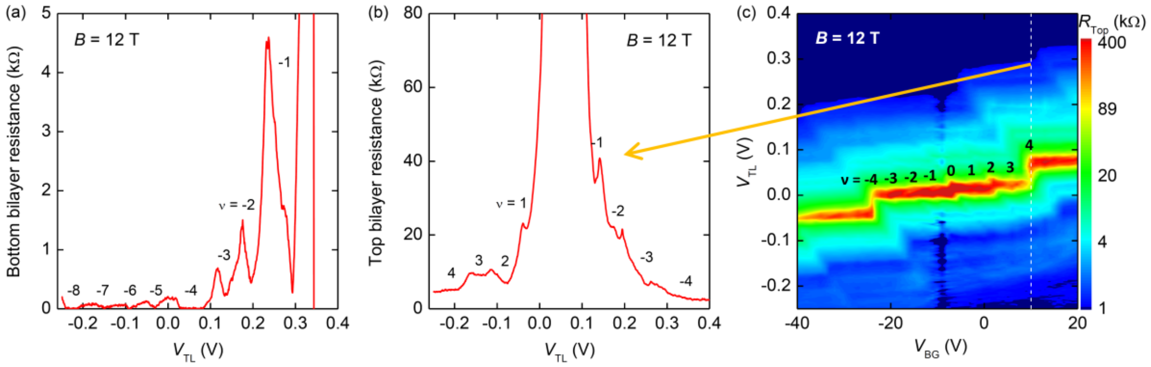


**Fig. S4.**

Longitudinal resistances of the (a) bottom and (b) top bilayer as a function of $V_{TL}$, in a magnetic field $B$ = 12 T. Broken symmetry integer quantum Hall states, identified by local minima, are marked. (c) Contour map of the top bilayer resistance ($R_{Top}$) as a function of $V_{BG}$ and $V_{TL}$, in $B$ = 12 T. The changes of $V_{TL}$ along the charge neutrality line (the red locus) represent the chemical potential change in the bottom bilayer graphene, in unit of eV.

Expected difference in energy drag between monolayer and bilayer graphene

We briefly discuss how the band structure differences between monolayer and bilayer graphene impact the energy drag. As addressed in the main text, the charge current $I$ and heat current $I_q$ obey the following relation $I_q = Q \cdot I$, where

$$Q = \frac{\pi^2 k_B{}^2 T^2}{3e} \frac{(d\sigma/d\mu)}{\sigma} \qquad \text{(S8)}$$

where $k_B$ is the Boltzmann's constant, and $\sigma$ is the layer conductivity. We approximate $\sigma = ne\mu_{FE} + \sigma_0$, where $\mu_{FE}$ is the layer mobility, and $\sigma_0$ is the conductivity at charge neutrality, determined by sample disorder and temperature. Using the linear energy-momentum dispersion for monolayer graphene, and the parabolic dispersion for bilayer graphene, Eq. (S8) then can be written as

$$Q = \alpha \frac{\pi^2 k_B{}^2 T^2}{3e} \frac{\mu}{\mu^2 + \delta^2} \qquad \text{(S9)}$$

Here, $\alpha = 2$ and $\delta^2 = \sigma_0 \hbar^2 \upsilon^2 \pi / e\mu_{FE}$ for monolayer graphene, $\upsilon$ is Fermi velocity and $\hbar$ is the reduced Planck's constant, and $\alpha = 1$ and $\delta^2 = \sigma_0 \hbar^2 \pi\mu / 2e\mu_{FE} m^*$ for bilayer graphene, $m^* = 0.034\ m_e$ is effective mass. Assuming nominal values $\sigma_0 = 2e^2/h$, $\upsilon = 10^6$ m/s, and $\mu_{FE} = 100{,}000$ cm$^2$/Vs provide $\delta^2 = 66$ meV$^2$ for monolayer graphene. By contrast, $\delta^2$ vanishes for bilayer graphene at charge neutrality. Consequently, for $T = 1.5$ K we obtain $\partial Q/\partial\mu|_{\mu=0} = -0.0017$ e$^{-1}$ in monolayer graphene, whereas $\partial Q/\partial\mu|_{\mu=0} = -1.9$ e$^{-1}$ in bilayer graphene, a value more than 1000 times larger compared to monolayer graphene.

The larger $\partial Q/\partial\mu$ leads to the giant energy drag at charge neutrality in bilayer graphene, a striking difference which originates from the larger density of states in bilayer graphene by comparison to monolayer graphene. We note that the value of $\partial Q/\partial\mu$ at charge neutrality, calculated using the measured $\sigma$ in bilayer graphene [Fig. 4(a)] is smaller than the above example, where the disorder-induced chemical potential fluctuations are neglected. To account for density fluctuations at charge neutrality, we substitute $\mu$ with an approximate potential fluctuation $\delta\mu = 5$ meV [S6], which yields $\delta^2 = 0.85$ meV$^2$ and $\partial Q/\partial\mu|_{\mu=0} = 0.06$ e$^{-1}$ for bilayer graphene, close to the value presented in Fig. 4(a).

The $T$-dependence of $\partial Q/\partial\mu$ can be simply written as $T^2/\delta^2$, where $\delta^2$ includes the $T$-dependency of $\sigma_0$. Approximating to $\delta^2 \approx \delta_0{}^2 + 6.25(k_B T)^2$ for both monolayer [S7], and zero gap bilayer graphene provides several order smaller $\delta_0{}^2 = 0.7$ meV$^2$ for bilayer graphene compared to that of monolayer graphene $\delta_0{}^2 = 66$ meV$^2$ at $T = 1.5$ K. The simple picture in energy drag, assuming the layer reciprocity in the active region as in [S7] and identical $\partial Q/\partial\mu$ for both bottom and top bilayer suggests the drag resistivity

$$\rho_{D,B} = \rho_{D,T} = \frac{1}{2T\kappa}\left(\frac{\partial Q}{\partial\mu}\right)^2 \sum_{\mathbf{q}} \frac{\langle \delta\mu_B(-\mathbf{q})\delta\mu_T(\mathbf{q})\rangle}{1 + \ell^2 q^2}, \qquad \text{(S10)}$$

$\kappa \propto \delta^2 T$ is thermal conductivity and $\ell$ is the interlayer cooling length, which is close to the inelastic mean free path. The $T$-dependence of drag resistivity is then given by $T^2/(\delta_0^2 + 6.25(k_B T)^2)^3$, a non-monotonic function which reaches a maximum at a temperature $T^*$, where a lower value of $\delta^2$ leads to a lower $T^*$. This estimate yields $T^* \sim 3$ K for double bilayer graphene system by comparison to $T^* \sim 50$ K using $\kappa \propto \delta^2/T$ [S7], valid at the $T >$ 50 K for double monolayer graphene.

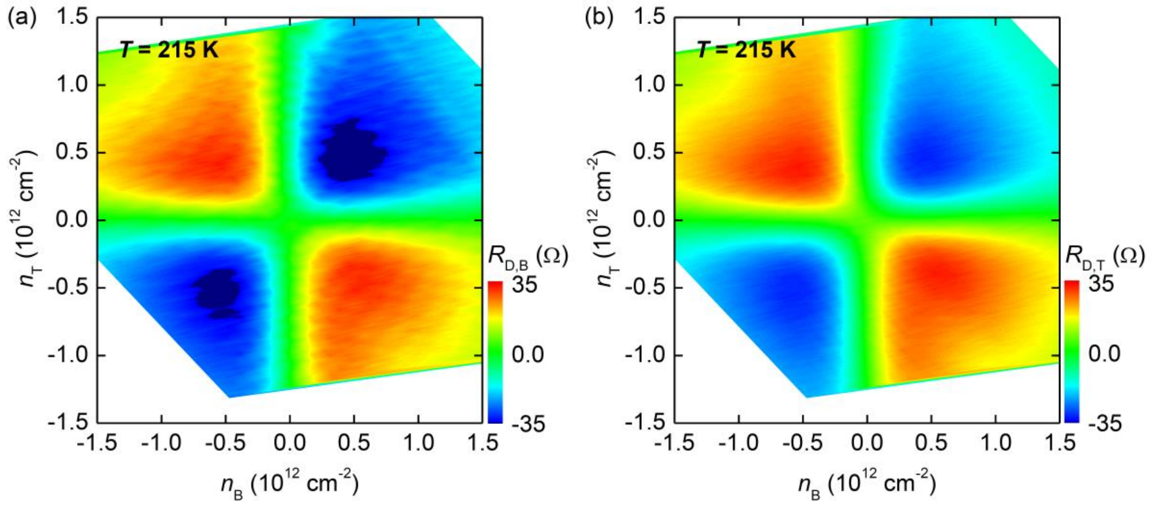


**Fig. S5.** Momentum exchange induced drag at elevated temperatures in double bilayer graphene heterostructures: Drag resistances measured in the bottom ($R_{D,B}$) and top ($R_{D,T}$) bilayer as a function of $n_B$ and $n_T$, at elevated $T$ = 215 K in Sample A. We observe positive (negative) drag when the drive and drag layer carrier types are opposite (equal), and similar magnitudes in $R_{D,B}$ and $R_{D,T}$, indicating that the layer reciprocity is obeyed.

Table S1. Sample specifications

| Sample | interlayer thickness (nm) | $C_{BG}$ (nF/cm$^2$) | $C_{int}$ (nF/cm$^2$) | Cool down | bottom bilayer mobility (cm$^2$/Vs) | top bilayer mobility (cm$^2$/Vs) | $E_{B0}$ (V/nm) | $E_{T0}$ (V/nm) |
|---|---|---|---|---|---|---|---|---|
| A | 3 | 11 | 840 | 1 | 180,000 – 260,000 | 51,000 – 68,000 | 0.04 | ~ 0.1 |
| | | | | 2 | 68,000 – 95,000 | 31,000 – 51,000 | 0.04 | ~ 0.1 |
| B | 2 | 11.58 | 1085 | 1 | 62,000 – 120,000 | 9,000 – 19000 | 0.11 | ~ 0 |
| C | 2 | 10.5 | 1097 | 1 | 180,000 – 210,000 | 3500 | 0.23 | ~ 0.25 |
| D | 5.5 | 10 | 430 | 1 | 100,000 – 110,000 | 3400 | 0.54 | ~ 0.5 |
| E | 2.7 | 11 | 900 | 1 | 24,000 | 2000 | ~ 0.35 | ~ 0.35 |

References


[S1] K. Lee, B. Fallahazad, J. Xue, D. C. Dillen, K. Kim, T. Taniguchi, K. Watanabe, and E. Tutuc, Science **345**, 58 (2014).

[S2] S. Kim and E. Tutuc, Solid State Commun. **152**, 1283 (2012).

[S3] B. Fallahazad *et al.*, Nano Letters **15**, 428 (2015).

[S4] K. Lee, B. Fallahazad, H. Min, and E. Tutuc, IEEE Transactions on Electron Devices **60**, 103 (2013).

[S5] E. McCann and V. I. Fal'ko, Phys. Rev. Lett. **96**, 086805 (2006).

[S6] J. Xue, J. Sanchez-Yamagishi, D. Bulmash, P. Jacquod, A. Deshpande, K. Watanabe, T. Taniguchi, P. Jarillo-Herrero, and B. J. LeRoy, Nature Mater. **10**, 282 (2011).

[S7] J. C. W. Song and L. S. Levitov, Phys. Rev. Lett. **109**, 236602 (2012).
